# Supplementary material for: Learning Preferences for Manipulation Tasks from Online Coactive Feedback
Source: arXiv:1601.00741 source file (2016-01-05)
Supplement: Supplementary file 1 [file supplementary.tex]

%%%%%%%%%%%%%%%%%%%% author.tex %%%%%%%%%%%%%%%%%%%%%%%%%%%%%%%%%%%
%
% sample root file for your "contribution" to a contributed volume
%
% Use this file as a template for your own input.
%
%%%%%%%%%%%%%%%% Springer %%%%%%%%%%%%%%%%%%%%%%%%%%%%%%%%%%%%%%%%%

%% RECOMMENDED %%%%%%%%%%%%%%%%%%%%%%%%%%%%%%%%%%%%%%%%%%%%%%%%%%%
\documentclass[graybox]{svmult}
%
%% choose options for [] as required from the list
% in the Reference Guide
%
\usepackage{relsize}
\usepackage{amssymb,amsmath}
\usepackage{url}
\usepackage[font=small,it]{caption}

\usepackage{enumitem}
\usepackage{xcolor}
\usepackage{verbatim}
\usepackage{caption}

\usepackage{times}
\usepackage{wrapfig,booktabs,blindtext}
\usepackage{color}
\usepackage{xcolor}
\usepackage{algorithm}
\usepackage{algorithmic}
\usepackage{mathptmx}       % selects Times Roman as basic font

%\usepackage{helvet}         % selects Helvetica as sans-serif font
%\usepackage{courier}        % selects Courier as typewriter font
%\usepackage{type1cm}        % activate if the above 3 fonts are
                             % not available on your system
%
\usepackage{makeidx}         % allows index generation
\usepackage{graphicx}        % standard LaTeX graphics tool
%                             % when including figure files
%\usepackage{multicol}        % used for the two-column index
\usepackage[bottom]{footmisc}% places footnotes at page bottom
%
%% see the list of further useful packages
%% in the Reference Guide
%
\usepackage{multirow}
\usepackage[numbers]{natbib}
\usepackage{subfigure}

\input{space_saver}
%\makeindex             % used for the subject index
%                       % please use the style svind.ist with
%                       % your makeindex program
%
%%%%%%%%%%%%%%%%%%%%%%%%%%%%%%%%%%%%%%%%%%%%%%%%%%%%%%%%%%%%%%%%%%%%%%%%%%%%%%%%%%%%%%%%%%
%

\begin{document}

% \chapter{}
%\title{To decide}
\title{Supplementary Material for: Learning Trajectory Preferences for Manipulators via Iterative Improvement}
% Use \titlerunning{Short Title} for an abbreviated version of
% your contribution title if the original one is too long
\author{Ashesh Jain, Shikhar Sharma and Ashutosh Saxena}
% Use \authorrunning{Short Title} for an abbreviated version of
% your contribution title if the original one is too long
\institute{Ashesh Jain, Shikhar Sharma, Ashutosh Saxena \at Department of Computer Science, Cornell University, Ithaca, New York.\\
 \email{{ashesh,ss2986,asaxena}@cs.cornell.edu}}
%
% Use the package "url.sty" to avoid
% problems with special characters
% used in your e-mail or web address
%
\maketitle

\section{Proof for Average Regret}
\input{expectation-proof}
\section{Proof for Expected Regret}
\input{expectation-proof-expt}

\setlength{\bibsep}{0pt}
{\small
\bibliographystyle{plainnat}
\bibliography{../COMTools/shortstrings,../COMTools/references}
}

\end{document}
